# Supplementary material for: Light-Hole Gate-Defined Spin-Orbit Qubit
Source: arXiv:2211.10514 ancillary file (2023-04-20)
Supplement: Supplementary file 1 [file supp.pdf]

# Light-Hole Gate-Defined Spin-Orbit Qubit

Patrick Del Vecchio and Oussama Moutanabbir*
*Department of Engineering Physics, École Polytechnique de Montréal,*
*Montréal, C.P. 6079, Succ. Centre-Ville, Montréal, Québec, Canada H3C 3A7*
(Dated: April 20, 2023)

## EIGHT-BAND $k \cdot p$ MATRIX

In this section, we present the $k \cdot p$ matrix in the cartesian representation

$$\{|S\uparrow\rangle, |S\downarrow\rangle, |X\uparrow\rangle, |Y\uparrow\rangle, |Z\uparrow\rangle, |X\downarrow\rangle, |Y\downarrow\rangle, |Z\downarrow\rangle\} \tag{1}$$

following the notation in Ref. [1, 2]. As mentioned in the main text, the total energy can be written as a sum of contributions. We have $H_{k\cdot p} = H_k + H_{\mathrm{SO}} + H_\varepsilon + H_B$ with

$$H_k = \begin{bmatrix} H^k_{cc} & \mathbb{1}_{2\times2} \otimes H^k_{cv} \\ \mathbb{1}_{2\times2} \otimes H^k_{vc} & \mathbb{1}_{2\times2} \otimes H^k_{vv} \end{bmatrix}, \tag{2}$$

where

$$H^k_{cc} = E_g + \sum_{\alpha=\{x,y,z\}} K_\alpha A K_\alpha + \frac{i\alpha_0}{2} \sum_{\alpha\beta\gamma} \epsilon_{\alpha\beta\gamma} \sigma_\alpha K_\beta (g - g_0) K_\gamma, \tag{3}$$

$$H^k_{cv} = \begin{bmatrix} PK_x & PK_y & PK_z \end{bmatrix}, \tag{4}$$

$$H^k_{vc} = H^{k\dagger}_{cv}, \tag{5}$$

$$\left(H^k_{vv}\right)_{i,j} = \begin{cases} \sum_\alpha K_\alpha M K_\alpha + K_i (L - M) K_i & i = j \\ K_i N_+ K_j + K_j N_- K_i & i \neq j \end{cases}. \tag{6}$$

where $E_g$ is the band gap energy and $g_0 \approx 2$. The parameters $L$, $M$ and $N_\pm$ are related to the Luttinger parameters and $\kappa$ by

$$\begin{bmatrix} L \\ M \\ N_+ + \alpha_0 \\ N_- - \alpha_0 \end{bmatrix} = -\alpha_0 \begin{bmatrix} 1 & 4 & 0 & 0 \\ 1 & -2 & 0 & 0 \\ 0 & 0 & 3 & 3 \\ 0 & 0 & 3 & -3 \end{bmatrix} \begin{bmatrix} \gamma_1 \\ \gamma_2 \\ \gamma_3 \\ \kappa \end{bmatrix}. \tag{7}$$

The parameters $A = \alpha_0 S$, $\gamma_{1,2,3}$, $\kappa$ and $g$ are rescaled versions of the parameters in $k \cdot p$ models with fewer bands [3]. The rescaling is proportional to the Kane matrix element $E_p = P^2/\alpha_0$ :

$$\gamma_1 = \gamma_1^{\mathrm{L}} - \frac{E_p}{3E_g} \tag{8}$$

$$\gamma_{2,3} = \gamma_{2,3}^{\mathrm{L}} - \frac{E_p}{6E_g} \tag{9}$$

$$\kappa = \kappa^{\mathrm{L}} - \frac{E_p}{6E_g} \tag{10}$$

$$g = g_c + \frac{2E_p}{3E_g} \frac{\Delta}{E_g + \Delta} \tag{11}$$

$$S = \frac{m_0}{m_c} - \frac{2E_p}{3E_g} \frac{3E_g/2 + \Delta}{E_g + \Delta}. \tag{12}$$

The spin-orbit interaction term $H_{\mathrm{SO}}$ is given by

$$H_{\mathrm{SO}} = \frac{\Delta}{3}\begin{bmatrix} 1 & 0 & 0 & 0 & 0 & 0 & 0 & 0 \\ 0 & 1 & 0 & 0 & 0 & 0 & 0 & 0 \\ 0 & 0 & 0 & -i & 0 & 0 & 0 & 1 \\ 0 & 0 & i & 0 & 0 & 0 & 0 & -i \\ 0 & 0 & 0 & 0 & 0 & -1 & i & 0 \\ 0 & 0 & 0 & 0 & -1 & 0 & i & 0 \\ 0 & 0 & 0 & 0 & -i & -i & 0 & 0 \\ 0 & 0 & 1 & i & 0 & 0 & 0 & 0 \end{bmatrix}. \tag{13}$$

The magnetic term $H_B$ is given by

$$H_B = \begin{bmatrix} H_B^k & 0 \\ 0 & H_B^k \otimes \mathbb{1}_{3\times 3} \end{bmatrix}, \tag{14}$$

with

$$H_B^k = \frac{i\alpha_0 g_0}{2} \sum_{\alpha\beta\gamma} \epsilon_{\alpha\beta\gamma} \sigma_\alpha K_\beta K_\gamma. \tag{15}$$

The strain term $H_\varepsilon$ is given by

$$H_\varepsilon = \begin{bmatrix} H_{cc}^\varepsilon & 0 \\ 0 & \mathbb{1}_{2\times 2} \otimes H_{vv}^\varepsilon \end{bmatrix}, \tag{16}$$

where

$$H_{cc}^\varepsilon = \mathbb{1}_{2\times 2} a_c \mathrm{Tr}\{\varepsilon\}, \tag{17}$$

$$(H_{vv}^\varepsilon)_{i,j} = \begin{cases} m\mathrm{Tr}\{\varepsilon\} + (l-m)\varepsilon_{ii} & i = j \\ n\varepsilon_{ij} & i \neq j \end{cases}. \tag{18}$$

Here the deformation potentials $l$, $m$, $n$ are related to the $a_v$, $b$ and $d$ parameters by

$$\begin{bmatrix} l \\ m \\ n \end{bmatrix} = \begin{bmatrix} 1 & 2 & 0 \\ 1 & -1 & 0 \\ 0 & 0 & \sqrt{3} \end{bmatrix} \begin{bmatrix} a_v \\ b \\ d \end{bmatrix}. \tag{19}$$

Finally, the potential energy $V(z)$ is the sum of the average valence band offset energies [4] with the potential associated with the external electric field :

$$V = E_{v,\mathrm{avg}} + eE_z z. \tag{20}$$

The change of basis from cartesian to the angular momentum representation [3]

$$\left\{ \left|\frac{1}{2},\frac{1}{2}\right\rangle_c, \left|\frac{3}{2},\frac{1}{2}\right\rangle, \left|\frac{1}{2},\frac{1}{2}\right\rangle, \left|\frac{3}{2},\frac{3}{2}\right\rangle, \left|\frac{1}{2},-\frac{1}{2}\right\rangle_c, \left|\frac{3}{2},-\frac{1}{2}\right\rangle, \left|\frac{1}{2},-\frac{1}{2}\right\rangle, \left|\frac{3}{2},-\frac{3}{2}\right\rangle \right\} \tag{21}$$

is performed by evaluating $U^\dagger H_{||} U$, where

$$U = \begin{bmatrix} 1 & 0 & 0 & 0 & 0 & 0 & 0 & 0 \\ 0 & 0 & 0 & 0 & 1 & 0 & 0 & 0 \\ 0 & 0 & 0 & -s_2 & 0 & s_6 & -s_3 & 0 \\ 0 & 0 & 0 & -is_2 & 0 & -is_6 & is_3 & 0 \\ 0 & s_{23} & -s_3 & 0 & 0 & 0 & 0 & 0 \\ 0 & -s_6 & -s_3 & 0 & 0 & 0 & 0 & s_2 \\ 0 & -is_6 & -is_3 & 0 & 0 & 0 & 0 & -is_2 \\ 0 & 0 & 0 & 0 & 0 & s_{23} & s_3 & 0 \end{bmatrix} \tag{22}$$

and $s_2 = 1/\sqrt{2}$, $s_3 = 1/\sqrt{3}$, $s_6 = 1/\sqrt{6}$ and $s_{23} = \sqrt{2/3}$. When evaluated at $K_x = K_y = 0$ and $B = 0$, $U^\dagger H_\| U$ has a block diagonal shape :

$$U^\dagger H_\|(\mathbf{K}_\| = 0, B = 0)U = \begin{bmatrix} H_+ & 0 \\ 0 & H_- \end{bmatrix}, \tag{23}$$

where

$$\begin{aligned} H_\sigma = V + \frac{\Delta}{3} + &\begin{bmatrix} E_g + k_z A k_z & \sqrt{2/3} P k_z & -\sigma P k_z/\sqrt{3} & 0 \\ \sqrt{2/3} k_z P & -\alpha_0 k_z(\gamma_1 + 2\gamma_2)k_z & 2\sqrt{2}\sigma\alpha_0 k_z \gamma_2 k_z & 0 \\ -\sigma k_z P/\sqrt{3} & 2\sqrt{2}\sigma\alpha_0 k_z\gamma_2 k_z & -\Delta - \alpha_0 k_z \gamma_1 k_z & 0 \\ 0 & 0 & 0 & -\alpha_0 k_z(\gamma_1 - 2\gamma_2)k_z \end{bmatrix} \\ + &\begin{bmatrix} a_c \mathrm{Tr}\{\varepsilon\} & 0 & 0 & 0 \\ 0 & a_v \mathrm{Tr}\{\varepsilon\} - b(\varepsilon_{xx} - \varepsilon_{zz}) & \sqrt{2}\sigma b(\varepsilon_{xx} - \varepsilon_{zz}) & 0 \\ 0 & \sqrt{2}\sigma b(\varepsilon_{xx} - \varepsilon_{zz}) & a_v \mathrm{Tr}\{\varepsilon\} & 0 \\ 0 & 0 & 0 & a_v \mathrm{Tr}\{\varepsilon\} + b(\varepsilon_{xx} - \varepsilon_{zz}) \end{bmatrix}. \end{aligned} \tag{24}$$

## $k \cdot p$ MATRIX IN SUBBAND EDGE BASIS

In this section we present the Hamiltonian for the in-plane motion of electrons and holes in the basis $\{|\eta\rangle, |\mathrm{H}\rangle\}$. Before that we need to introduce a few parameters. We first define the following superpositions of LH and SO envelopes :

$$|j\rangle_+ = |j\rangle_\ell + \sqrt{2}\,|j\rangle_s \tag{25}$$

$$|j\rangle_- = |j\rangle_\ell - 1/\sqrt{2}\,|j\rangle_s\,. \tag{26}$$

The orthonormality of the basis $\{|\eta\rangle, |\mathrm{H}\rangle\}$ implies

$$_c\langle j\,|\,j'\rangle_c + {}_\ell\langle j\,|\,j'\rangle_\ell + {}_s\langle j\,|\,j'\rangle_s = \delta_{j,j'}, \tag{27}$$

$$_h\langle l\,|\,l'\rangle_h = \delta_{l,l'}. \tag{28}$$

Next we define the matrices $\boldsymbol{\gamma}^{\mathrm{H}}$, $\boldsymbol{\gamma}^{\eta}$, $\mathbf{g}^{\mathrm{H}}$, $\mathbf{g}^{\eta}$, $\mathbf{R}$, $\mathbf{P}$, $\boldsymbol{\mu}$ and $\boldsymbol{\delta}$ whose elements are given by :

$$\gamma^{\mathrm{H}}_{l,l'} = -\,{}_h\langle l\,|\,\gamma_1+\gamma_2\,|\,l'\rangle_h \tag{29}$$

$$\gamma^{\eta}_{j,j'} = \frac{1}{\alpha_0}\,{}_c\langle j\,|\,A\,|\,j'\rangle_c - \frac{1}{3}\left(2\,{}_-\langle j\,|\,\gamma_1-2\gamma_2\,|\,j'\rangle_- + {}_+\langle j\,|\,\gamma_1+\gamma_2\,|\,j'\rangle_+\right) \tag{30}$$

$$g^{\mathrm{H}}_{l,l'} = -6\,{}_h\langle l\,|\,\kappa\,|\,l'\rangle_h \tag{31}$$

$$g^{\eta}_{j,j'} = {}_c\langle j\,|\,g-2\,|\,j'\rangle_c - 2\,{}_+\langle j\,|\,\kappa+1\,|\,j'\rangle_+ + 2\delta_{j,j'} \tag{32}$$

$$\begin{aligned} R_{j,j'} = &\frac{1}{\sqrt{6}}\left({}_c\langle j\,|\,P\,|\,j'\rangle_+ - {}_+\langle j\,|\,P\,|\,j'\rangle_c\right) \\ &-\alpha_0\left(\frac{1}{2}\,{}_c\langle j\,|\,[g,k_z]\,|\,j'\rangle_c - {}_+\langle j\,|\,q_+\,|\,j'\rangle_- + {}_-\langle j\,|\,q_-\,|\,j'\rangle_+\right)\end{aligned} \tag{33}$$

$$P_{j,l} = \left({}_c\langle j|\,P/\sqrt{2} - \sqrt{3}\alpha_0\,{}_-\langle j|\,q_-\right)|l\rangle_h \tag{34}$$

$$\mu_{j,l} = \sqrt{3}\,{}_+\langle j\,|\,\mu\,|\,l\rangle_h \tag{35}$$

$$\delta_{j,l} = \sqrt{3}\,{}_+\langle j\,|\,\delta\,|\,l\rangle_h\,, \tag{36}$$

with $q_\pm = \{\gamma_3, k_z\} \pm [\kappa, k_z]$, $\{X, Y\} = XY + YX$ is the anti-commutator, $\mu = (\gamma_2+\gamma_3)/2$ and $\delta = (\gamma_2-\gamma_3)/2$. Braket products are integrals of position-dependent material parameters with envelope functions along the growth direction, e.g.

$${}_c\langle j\,|\,g-2\,|\,j'\rangle_c = \int \psi^c_j(z)^*(g(z)-2)\psi^c_{j'}(z)dz, \tag{37}$$

where $\psi^c_j(z) = \langle z\,|\,j\rangle_c$. We also define diagonal matrices $\mathbf{E}^\eta$ and $\mathbf{E}^{\mathrm{H}}$ that contain all the subband energies $E^\eta_j$ and $E^{\mathrm{H}}_l$ respectively, at $\mathbf{K}_\parallel = 0$ and $B = 0$. In the orthonormal basis $\{|\eta,+\rangle, |\eta,-\rangle, |\mathrm{H},+\rangle, |\mathrm{H},-\rangle\}$, the Hamiltonian $H_\parallel$ for the in-plane motion reads :

$$H_\parallel = \begin{bmatrix} \mathbf{E}^\eta & 0 & 0 & 0 \\ 0 & \mathbf{E}^\eta & 0 & 0 \\ 0 & 0 & \mathbf{E}^{\mathrm{H}} & 0 \\ 0 & 0 & 0 & \mathbf{E}^{\mathrm{H}} \end{bmatrix} + \begin{bmatrix} \alpha_0\boldsymbol{\gamma}^\eta K_\parallel^2 + \frac{1}{2}\frac{\alpha_0}{\lambda^2}\mathbf{g}^\eta & \mathbf{R}K_- & -\mathbf{P}K_+ & \alpha_0\boldsymbol{\mu}K_-^2 + \alpha_0\boldsymbol{\delta}K_+^2 \\ & \alpha_0\boldsymbol{\gamma}^\eta K_\parallel^2 - \frac{1}{2}\frac{\alpha_0}{\lambda^2}\mathbf{g}^\eta & \alpha_0\boldsymbol{\mu}K_+^2 + \alpha_0\boldsymbol{\delta}K_-^2 & \mathbf{P}K_- \\ \dagger & & \alpha_0\boldsymbol{\gamma}^{\mathrm{H}} K_\parallel^2 + \frac{1}{2}\frac{\alpha_0}{\lambda^2}\mathbf{g}^{\mathrm{H}} & 0 \\ & & & \alpha_0\boldsymbol{\gamma}^{\mathrm{H}} K_\parallel^2 - \frac{1}{2}\frac{\alpha_0}{\lambda^2}\mathbf{g}^{\mathrm{H}} \end{bmatrix}. \tag{38}$$

The diagonal elements of the matrices $\boldsymbol{\gamma}^{\mathrm{H}}$, $\boldsymbol{\gamma}^\eta$, $\mathbf{g}^{\mathrm{H}}$, $\mathbf{g}^\eta$ represent the masses and $g$-factors of all the H and $\eta$ subbands respectively, to 1st order in perturbation. The matrix $\mathbf{R}$ represents couplings within $\eta$ subbands. The three other matrices $\mathbf{P}$, $\boldsymbol{\mu}$ and $\boldsymbol{\delta}$ represent LH-HH mixing. In our framework, electrons and holes use the same energy scale. This means that we associate an upwards parabolic dispersion (positive curvature) with a positive effective mass, regardless of whether it is an electron or a hole dispersion. Similarly, the $g$-factor sign is given by the energy difference $E_+ - E_-$ for both electrons and holes.

## PARAMETERS IN EFFECTIVE LH HAMILTONIAN

In this section we give the expressions for $\tilde{\gamma}$, $\tilde{\gamma}'$, $\tilde{g}$, $\tilde{g}'$, $\gamma_\lambda$, $\zeta$, $\beta_1$, $\beta_2$ and $\beta_3$ from 4th order perturbation theory. As long $H_{\mathrm{eff}}$ is quartic in $K$, no additional accuracy is gained by including the 5th order perturbation terms or higher, because the resulting corrections would be at least quintic in $K$. The linear Rashba coefficient $\beta_1$ for the $j$-th $\eta$ subband is given directly from 1st order perturbation :

$$\beta_1 = -iR_{j,j}. \tag{39}$$

An accurate formula for all the other parameters require at least 2nd order perturbation theory. We will use a compact notation to represent sums that are common in perturbation theory. This notation will be useful as some of the effective parameters have very lengthy expressions. We first define matrices that represent energy differences between $\eta$ and H subbands : $\mathbf{\Delta}_{\eta\eta}$ and $\mathbf{\Delta}_{\eta\mathrm{H}}$. The matrix elements are, respectively :

$$\Delta^{\eta\eta}_{j,j'} = E^{\eta}_{j} - E^{\eta}_{j'}, \tag{40}$$

$$\Delta^{\eta\mathrm{H}}_{j,l} = E^{\eta}_{j} - E^{\mathrm{H}}_{l}. \tag{41}$$

The effective mass parameter $\tilde{\gamma}$, the effective $g$-factor $\tilde{g}$ and the cubic Rashba parameter $\beta_2$ for the $j$-th $\eta$ subband require only 2nd order perturbation. They have the following expression in compact notation :

$$\tilde{\gamma} = \gamma^{\eta}_{j,j} - \frac{1}{\alpha_0}\left(\frac{\mathbf{RR}}{\mathbf{\Delta}_{\eta\eta}} - \frac{\mathbf{PP}^{\dagger}}{\mathbf{\Delta}_{\eta\mathrm{H}}}\right), \tag{42}$$

$$\tilde{g} = g^{\eta}_{j,j} - \frac{2}{\alpha_0}\left(\frac{\mathbf{RR}}{\mathbf{\Delta}_{\eta\eta}} + \frac{\mathbf{PP}^{\dagger}}{\mathbf{\Delta}_{\eta\mathrm{H}}}\right), \tag{43}$$

$$\beta_2 = -2\alpha_0 \Im\left\{\frac{\boldsymbol{\delta}\mathbf{P}^{\dagger}}{\mathbf{\Delta}_{\eta\mathrm{H}}}\right\}. \tag{44}$$

Here the fractions involving matrices represent sums :

$$\frac{\mathbf{RR}}{\mathbf{\Delta}_{\eta\eta}} \equiv \sum_{j'\neq j} \frac{R_{j,j'}R_{j',j}}{E^{\eta}_{j} - E^{\eta}_{j'}}, \tag{45}$$

$$\frac{\mathbf{PP}^{\dagger}}{\mathbf{\Delta}_{\eta\mathrm{H}}} \equiv \sum_{l} \frac{P_{j,l}P^{*}_{j,l}}{E^{\eta}_{j} - E^{\mathrm{H}}_{l}}, \tag{46}$$

$$\frac{\boldsymbol{\delta}\mathbf{P}^{\dagger}}{\mathbf{\Delta}_{\eta\mathrm{H}}} \equiv \sum_{l} \frac{\delta_{j,l}P^{*}_{j,l}}{E^{\eta}_{j} - E^{\mathrm{H}}_{l}}. \tag{47}$$

The anisotropy parameter $\zeta$ and the cubic Rashba coefficient $\beta_3$ require 3rd order perturbation. They have the following expression in compact notation :

$$\zeta = \frac{\boldsymbol{\mu}\boldsymbol{\delta}^{\dagger}}{\mathbf{\Delta}_{\eta\mathrm{H}}} - \frac{\beta_1}{\alpha_0}\Im\left\{\frac{\boldsymbol{\delta}\mathbf{P}^{\dagger}}{\mathbf{\Delta}^{2}_{\eta\mathrm{H}}}\right\} + \frac{1}{\alpha_0}\left(\frac{\mathbf{RP}\boldsymbol{\delta}^{\dagger}}{\mathbf{\Delta}_{\eta\eta}\mathbf{\Delta}_{\eta\mathrm{H}}} - \frac{\mathbf{R}\boldsymbol{\delta}\mathbf{P}^{\dagger}}{\mathbf{\Delta}_{\eta\eta}\mathbf{\Delta}_{\eta\mathrm{H}}}\right), \tag{48}$$

$$\beta_3 = 2\alpha_0\Im\left\{\frac{\boldsymbol{\gamma}^{\eta}\mathbf{R}}{\mathbf{\Delta}_{\eta\eta}} + \frac{\boldsymbol{\mu}\mathbf{P}^{\dagger}}{\mathbf{\Delta}_{\eta\mathrm{H}}}\right\} + \beta_1\left(\frac{\mathbf{RR}}{\mathbf{\Delta}^{2}_{\eta\eta}} - \frac{\mathbf{PP}^{\dagger}}{\mathbf{\Delta}^{2}_{\eta\mathrm{H}}}\right) + i\frac{\mathbf{RRR}}{\mathbf{\Delta}_{\eta\eta}\mathbf{\Delta}_{\eta\eta}} + 2\Im\left\{\frac{\mathbf{RPP}^{\dagger}}{\mathbf{\Delta}_{\eta\eta}\mathbf{\Delta}_{\eta\mathrm{H}}}\right\}. \tag{49}$$

Note how $\zeta$ and $\beta_2$ are directly proportional to $\delta$ and thus vanish in the axial approximation, where $\gamma_2 = \gamma_3$ is assumed. Here are few examples on how the compact notation expands to sums :

$$\frac{\boldsymbol{\delta}\mathbf{P}^{\dagger}}{\mathbf{\Delta}^{2}_{\eta\mathrm{H}}} \equiv \sum_{l} \frac{\delta_{j,l}P^{*}_{j,l}}{\left(E^{\eta}_{j} - E^{\mathrm{H}}_{l}\right)^{2}}, \tag{50}$$

$$\frac{\mathbf{RP}\boldsymbol{\delta}^{\dagger}}{\mathbf{\Delta}_{\eta\eta}\mathbf{\Delta}_{\eta\mathrm{H}}} \equiv \sum_{j'\neq j}\sum_{l} \frac{R_{j,j'}P_{j',l}\delta^{*}_{j,l}}{\left(E^{\eta}_{j} - E^{\eta}_{j'}\right)\left(E^{\eta}_{j} - E^{\mathrm{H}}_{l}\right)}, \tag{51}$$

$$\frac{\mathbf{RRR}}{\mathbf{\Delta}_{\eta\eta}\mathbf{\Delta}_{\eta\eta}} \equiv \sum_{j'\neq j}\sum_{j''\neq j} \frac{R_{j,j'}R_{j',j''}R_{j'',j}}{\left(E^{\eta}_{j} - E^{\eta}_{j'}\right)\left(E^{\eta}_{j} - E^{\eta}_{j''}\right)}. \tag{52}$$

Other terms expand in a similar way. The non-linear parameters $\tilde{\gamma}'$, $\tilde{g}'$ and $\gamma_\lambda$ require 4th order perturbation theory :

$$
\begin{aligned}
\tilde{\gamma}' = &\frac{\boldsymbol{\gamma}^\eta\boldsymbol{\gamma}^\eta}{\boldsymbol{\Delta}_{\eta\eta}} + \frac{\boldsymbol{\mu}\boldsymbol{\mu}^\dagger}{\boldsymbol{\Delta}_{\eta\mathrm{H}}} + \frac{\boldsymbol{\delta}\boldsymbol{\delta}^\dagger}{\boldsymbol{\Delta}_{\eta\mathrm{H}}} + \frac{1}{\alpha_0}\left[2iR_{j,j}\Im\left\{\frac{\boldsymbol{\gamma}^\eta\mathbf{R}}{\boldsymbol{\Delta}^2_{\eta\eta}} + \frac{\boldsymbol{\mu}\mathbf{P}^\dagger}{\boldsymbol{\Delta}^2_{\eta\mathrm{H}}}\right\} + \gamma^\eta_{j,j}\left(\frac{\mathbf{R}\mathbf{R}}{\boldsymbol{\Delta}^2_{\eta\eta}} - \frac{\mathbf{P}\mathbf{P}^\dagger}{\boldsymbol{\Delta}^2_{\eta\mathrm{H}}}\right)\right.\\
&\left.-\frac{\mathbf{R}\boldsymbol{\gamma}^\eta\mathbf{R}}{\boldsymbol{\Delta}_{\eta\eta}\boldsymbol{\Delta}_{\eta\eta}} + \frac{\mathbf{P}\boldsymbol{\gamma}^\mathrm{H}\mathbf{P}^\dagger}{\boldsymbol{\Delta}_{\eta\mathrm{H}}\boldsymbol{\Delta}_{\eta\mathrm{H}}} - 2\Re\left\{\frac{\boldsymbol{\gamma}^\eta\mathbf{R}\mathbf{R}}{\boldsymbol{\Delta}_{\eta\eta}\boldsymbol{\Delta}_{\eta\eta}} - \frac{\boldsymbol{\gamma}^\eta\mathbf{P}\mathbf{P}^\dagger}{\boldsymbol{\Delta}_{\eta\eta}\boldsymbol{\Delta}_{\eta\mathrm{H}}} - \frac{\mathbf{R}\mathbf{P}\boldsymbol{\mu}^\dagger}{\boldsymbol{\Delta}_{\eta\eta}\boldsymbol{\Delta}_{\eta\mathrm{H}}} - \frac{\mathbf{P}\boldsymbol{\mu}^\dagger\mathbf{R}}{\boldsymbol{\Delta}_{\eta\mathrm{H}}\boldsymbol{\Delta}_{\eta\eta}}\right\}\right]\\
&+\frac{1}{\alpha_0^2}\left[R^2_{j,j}\left(\frac{\mathbf{R}\mathbf{R}}{\boldsymbol{\Delta}^3_{\eta\eta}} - \frac{\mathbf{P}\mathbf{P}^\dagger}{\boldsymbol{\Delta}^3_{\eta\mathrm{H}}}\right) + 2iR_{j,j}\Im\left\{\frac{\mathbf{R}\mathbf{P}\mathbf{P}^\dagger}{\boldsymbol{\Delta}^2_{\eta\eta}\boldsymbol{\Delta}_{\eta\mathrm{H}}} + \frac{\mathbf{R}\mathbf{P}\mathbf{P}^\dagger}{\boldsymbol{\Delta}_{\eta\eta}\boldsymbol{\Delta}^2_{\eta\mathrm{H}}} - \frac{\mathbf{R}\mathbf{R}\mathbf{R}}{\boldsymbol{\Delta}^2_{\eta\eta}\boldsymbol{\Delta}_{\eta\eta}}\right\} + \frac{\mathbf{R}\mathbf{R}}{\boldsymbol{\Delta}^2_{\eta\eta}}\frac{\mathbf{P}\mathbf{P}^\dagger}{\boldsymbol{\Delta}_{\eta\mathrm{H}}} - \frac{\mathbf{R}\mathbf{R}}{\boldsymbol{\Delta}_{\eta\eta}}\frac{\mathbf{P}\mathbf{P}^\dagger}{\boldsymbol{\Delta}^2_{\eta\mathrm{H}}}\right.\\
&\left.+\frac{1}{2}\frac{\mathbf{R}\mathbf{R}\mathbf{R}\mathbf{R}}{\boldsymbol{\Delta}_{\eta\eta}\boldsymbol{\Delta}_{\eta\eta}\boldsymbol{\Delta}_{\eta\eta}} + \frac{1}{2}\frac{\mathbf{P}\mathbf{P}^\dagger\mathbf{P}\mathbf{P}^\dagger}{\boldsymbol{\Delta}_{\eta\mathrm{H}}\boldsymbol{\Delta}_{\eta\eta}\boldsymbol{\Delta}_{\eta\mathrm{H}}} - \frac{1}{2}\frac{\mathbf{R}\mathbf{P}\mathbf{P}^\dagger\mathbf{R}}{\boldsymbol{\Delta}_{\eta\eta}\boldsymbol{\Delta}_{\eta\mathrm{H}}\boldsymbol{\Delta}_{\eta\eta}} - \Re\left\{\frac{\mathbf{R}\mathbf{R}\mathbf{P}\mathbf{P}^\dagger}{\boldsymbol{\Delta}_{\eta\eta}\boldsymbol{\Delta}_{\eta\eta}\boldsymbol{\Delta}_{\eta\mathrm{H}}}\right\}\right]
\end{aligned}
\tag{53}
$$

$$
\begin{aligned}
\tilde{g}' = &\frac{1}{4}\frac{\mathbf{g}^\eta\mathbf{g}^\eta}{\boldsymbol{\Delta}_{\eta\eta}} + \frac{3\boldsymbol{\mu}\boldsymbol{\mu}^\dagger}{\boldsymbol{\Delta}_{\eta\mathrm{H}}} + \frac{3\boldsymbol{\delta}\boldsymbol{\delta}^\dagger}{\boldsymbol{\Delta}_{\eta\mathrm{H}}} + \frac{1}{\alpha_0}\left[2iR_{j,j}\Im\left\{\frac{\boldsymbol{\gamma}^\eta\mathbf{R}}{\boldsymbol{\Delta}^2_{\eta\eta}} + \frac{\boldsymbol{\mu}\mathbf{P}^\dagger}{\boldsymbol{\Delta}^2_{\eta\mathrm{H}}}\right\} + \frac{g^\eta_{j,j}}{2}\left(\frac{\mathbf{R}\mathbf{R}}{\boldsymbol{\Delta}^2_{\eta\eta}} + \frac{\mathbf{P}\mathbf{P}^\dagger}{\boldsymbol{\Delta}^2_{\eta\mathrm{H}}}\right)\right.\\
&\left.-\frac{\mathbf{R}(2\boldsymbol{\gamma}^\eta - \mathbf{g}^\eta/2)\mathbf{R}}{\boldsymbol{\Delta}_{\eta\eta}\boldsymbol{\Delta}_{\eta\eta}} + \frac{\mathbf{P}(2\boldsymbol{\gamma}^\mathrm{H} - \mathbf{g}^\mathrm{H}/2)\mathbf{P}^\dagger}{\boldsymbol{\Delta}_{\eta\mathrm{H}}\boldsymbol{\Delta}_{\eta\mathrm{H}}} - \Re\left\{\frac{\mathbf{g}^\eta\mathbf{R}\mathbf{R}}{\boldsymbol{\Delta}_{\eta\eta}\boldsymbol{\Delta}_{\eta\eta}} + \frac{\mathbf{g}^\eta\mathbf{P}\mathbf{P}^\dagger}{\boldsymbol{\Delta}_{\eta\eta}\boldsymbol{\Delta}_{\eta\mathrm{H}}} - \frac{6\mathbf{R}\mathbf{P}\boldsymbol{\mu}^\dagger}{\boldsymbol{\Delta}_{\eta\eta}\boldsymbol{\Delta}_{\eta\mathrm{H}}} + \frac{2\mathbf{P}\boldsymbol{\mu}^\dagger\mathbf{R}}{\boldsymbol{\Delta}_{\eta\mathrm{H}}\boldsymbol{\Delta}_{\eta\eta}}\right\}\right]\\
&+\frac{1}{\alpha_0^2}\left[R^2_{j,j}\left(\frac{\mathbf{R}\mathbf{R}}{\boldsymbol{\Delta}^3_{\eta\eta}} + \frac{\mathbf{P}\mathbf{P}^\dagger}{\boldsymbol{\Delta}^3_{\eta\mathrm{H}}}\right) + 2iR_{j,j}\Im\left\{\frac{\mathbf{R}\mathbf{P}\mathbf{P}^\dagger}{\boldsymbol{\Delta}^2_{\eta\eta}\boldsymbol{\Delta}_{\eta\mathrm{H}}} + \frac{\mathbf{R}\mathbf{P}\mathbf{P}^\dagger}{\boldsymbol{\Delta}_{\eta\eta}\boldsymbol{\Delta}^2_{\eta\mathrm{H}}} - \frac{\mathbf{R}\mathbf{R}\mathbf{R}}{\boldsymbol{\Delta}^2_{\eta\eta}\boldsymbol{\Delta}_{\eta\eta}}\right\} - \frac{\mathbf{R}\mathbf{R}}{\boldsymbol{\Delta}^2_{\eta\eta}}\frac{\mathbf{P}\mathbf{P}^\dagger}{\boldsymbol{\Delta}_{\eta\mathrm{H}}} - \frac{\mathbf{R}\mathbf{R}}{\boldsymbol{\Delta}_{\eta\eta}}\frac{\mathbf{P}\mathbf{P}^\dagger}{\boldsymbol{\Delta}^2_{\eta\mathrm{H}}}\right.\\
&\left.+\frac{1}{2}\frac{\mathbf{R}\mathbf{R}\mathbf{R}\mathbf{R}}{\boldsymbol{\Delta}_{\eta\eta}\boldsymbol{\Delta}_{\eta\eta}\boldsymbol{\Delta}_{\eta\eta}} + \frac{1}{2}\frac{\mathbf{P}\mathbf{P}^\dagger\mathbf{P}\mathbf{P}^\dagger}{\boldsymbol{\Delta}_{\eta\mathrm{H}}\boldsymbol{\Delta}_{\eta\eta}\boldsymbol{\Delta}_{\eta\mathrm{H}}} - \frac{3}{2}\frac{\mathbf{R}\mathbf{P}\mathbf{P}^\dagger\mathbf{R}}{\boldsymbol{\Delta}_{\eta\eta}\boldsymbol{\Delta}_{\eta\mathrm{H}}\boldsymbol{\Delta}_{\eta\eta}} + \Re\left\{\frac{\mathbf{R}\mathbf{R}\mathbf{P}\mathbf{P}^\dagger}{\boldsymbol{\Delta}_{\eta\eta}\boldsymbol{\Delta}_{\eta\eta}\boldsymbol{\Delta}_{\eta\mathrm{H}}}\right\}\right]
\end{aligned}
\tag{54}
$$

$$
\begin{aligned}
\gamma_\lambda = &\Re\left\{\frac{\boldsymbol{\gamma}^\eta\mathbf{g}^\eta}{\boldsymbol{\Delta}_{\eta\eta}}\right\} + \frac{4\boldsymbol{\mu}\boldsymbol{\mu}^\dagger}{\boldsymbol{\Delta}_{\eta\mathrm{H}}} - \frac{4\boldsymbol{\delta}\boldsymbol{\delta}^\dagger}{\boldsymbol{\Delta}_{\eta\mathrm{H}}} + \frac{1}{\alpha_0}\left[4iR_{j,j}\Im\left\{\frac{\boldsymbol{\gamma}^\eta\mathbf{R}}{\boldsymbol{\Delta}^2_{\eta\eta}} + \frac{\boldsymbol{\mu}\mathbf{P}^\dagger}{\boldsymbol{\Delta}^2_{\eta\mathrm{H}}}\right\} + \gamma^\eta_{j,j}\left(\frac{\mathbf{R}\mathbf{R}}{\boldsymbol{\Delta}^2_{\eta\eta}} + \frac{\mathbf{P}\mathbf{P}^\dagger}{\boldsymbol{\Delta}^2_{\eta\mathrm{H}}}\right) + \frac{g^\eta_{j,j}}{2}\left(\frac{\mathbf{R}\mathbf{R}}{\boldsymbol{\Delta}^2_{\eta\eta}} - \frac{\mathbf{P}\mathbf{P}^\dagger}{\boldsymbol{\Delta}^2_{\eta\mathrm{H}}}\right)\right.\\
&\left.-\frac{\mathbf{R}(3\boldsymbol{\gamma}^\eta - \mathbf{g}^\eta/2)\mathbf{R}}{\boldsymbol{\Delta}_{\eta\eta}\boldsymbol{\Delta}_{\eta\eta}} - \frac{\mathbf{P}(3\boldsymbol{\gamma}^\mathrm{H} - \mathbf{g}^\mathrm{H}/2)\mathbf{P}^\dagger}{\boldsymbol{\Delta}_{\eta\mathrm{H}}\boldsymbol{\Delta}_{\eta\mathrm{H}}} - 2\Re\left\{\frac{(\boldsymbol{\gamma}^\eta + \mathbf{g}^\eta/2)\mathbf{R}\mathbf{R}}{\boldsymbol{\Delta}_{\eta\eta}\boldsymbol{\Delta}_{\eta\eta}} + \frac{(\boldsymbol{\gamma}^\eta - \mathbf{g}^\eta/2)\mathbf{P}\mathbf{P}^\dagger}{\boldsymbol{\Delta}_{\eta\eta}\boldsymbol{\Delta}_{\eta\mathrm{H}}} - \frac{4\mathbf{R}\mathbf{P}\boldsymbol{\mu}^\dagger}{\boldsymbol{\Delta}_{\eta\eta}\boldsymbol{\Delta}_{\eta\mathrm{H}}}\right\}\right]\\
&+\frac{1}{\alpha_0^2}\left[2R^2_{j,j}\frac{\mathbf{R}\mathbf{R}}{\boldsymbol{\Delta}^3_{\eta\eta}} + 4iR_{j,j}\Im\left\{\frac{\mathbf{R}\mathbf{P}\mathbf{P}^\dagger}{\boldsymbol{\Delta}^2_{\eta\eta}\boldsymbol{\Delta}_{\eta\mathrm{H}}} + \frac{\mathbf{R}\mathbf{P}\mathbf{P}^\dagger}{\boldsymbol{\Delta}_{\eta\eta}\boldsymbol{\Delta}^2_{\eta\mathrm{H}}} - \frac{\mathbf{R}\mathbf{R}\mathbf{R}}{\boldsymbol{\Delta}^2_{\eta\eta}\boldsymbol{\Delta}_{\eta\eta}}\right\}\right.\\
&\left.+\frac{\mathbf{R}\mathbf{R}\mathbf{R}\mathbf{R}}{\boldsymbol{\Delta}_{\eta\eta}\boldsymbol{\Delta}_{\eta\eta}\boldsymbol{\Delta}_{\eta\eta}} - \frac{\mathbf{P}\mathbf{P}^\dagger\mathbf{P}\mathbf{P}^\dagger}{\boldsymbol{\Delta}_{\eta\mathrm{H}}\boldsymbol{\Delta}_{\eta\eta}\boldsymbol{\Delta}_{\eta\mathrm{H}}} - \frac{2\mathbf{R}\mathbf{P}\mathbf{P}^\dagger\mathbf{R}}{\boldsymbol{\Delta}_{\eta\eta}\boldsymbol{\Delta}_{\eta\mathrm{H}}\boldsymbol{\Delta}_{\eta\eta}}\right]
\end{aligned}
\tag{55}
$$

As a complement to the equations given above, we show the dependence of the effective mass parameter $\tilde{\gamma}$ and $g$-factor $\tilde{g}$ for different quantum well parameters in Fig. 1. The region of opposite sign effective mass is clearly visible in panel (a). We also observe a rise in the $g$-factor value with decreasing QW thickness, which we attribute to a larger $\eta$-H mixing due to the proximity of the ground LH subband with the HH barrier states.

## SOLUTION OF TIME-INDEPENDENT QUANTUM DOT HAMILTONIAN

In this section we diagonalize the time-independent quantum dot Hamiltonian $H_{\mathrm{QD}}$. We divide this task in two parts : first we diagonalize $H_0$, that is, $H_{\mathrm{QD}}$ without the spin-orbit coupling term $H'$. Then we take in account $H'$ by using the solutions from the $H_0$ part.

The Hamiltonian of the quantum dot without spin-orbit coupling is given by eq. (3) in the main text :

$$
H_0 = \alpha_0\tilde{\gamma}K_\parallel^2 + \frac{1}{2}m^*\omega_0^2\left(x^2+y^2\right) + \frac{\alpha_0}{\lambda^2}\frac{\tilde{g}}{2}\sigma_z. \tag{56}
$$

This Hamiltonian can be diagonalized analytically by defining the following ladder operators :

$$
a_1 = \frac{x-iy}{2r} + \frac{irk_-}{2}, \qquad a_2 = \frac{x+iy}{2r} + \frac{irk_+}{2}, \tag{57}
$$

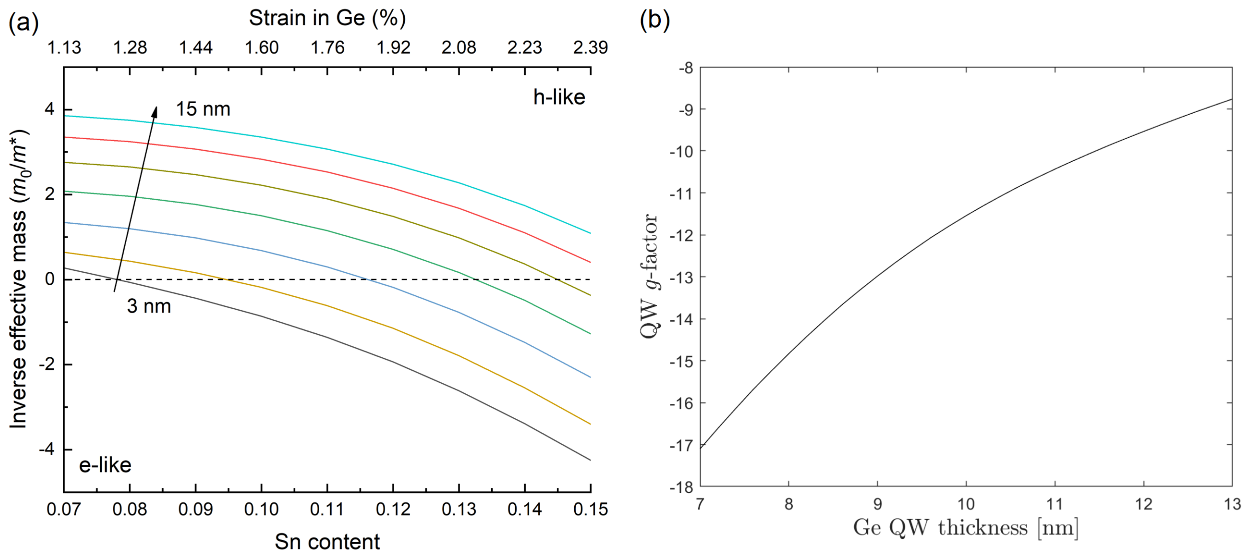


FIG. 1. (a) Effective mass parameter $\tilde{\gamma}$ and (b) effective $g$-factor $\tilde{g}$ as a function of the barrier Sn content.

where $k_\pm = k_x \pm ik_y$, $r = \sqrt{\hbar/(m^*\omega_l)}$ is the effective quantum dot radius, $\omega_l^2 = \omega_0^2 + \omega_c^2/4$ and $\omega_c = eB/m^*$ is the cyclotron frequency. It is useful to define the dot radius at zero magnetic field $r_0 = \sqrt{\hbar/(m^*\omega_0)}$, which is related to $r$ by

$$\frac{1}{r^4} = \frac{1}{r_0^4} + \frac{1}{4\lambda^4}. \tag{58}$$

The ladder operators $a_1$ and $a_2$ follow the usual commutation relations for bosons : $[a_i, a_j] = [a_i^\dagger, a_j^\dagger] = 0$ and $[a_i, a_j^\dagger] = \delta_{i,j}$. They also act upon the eigenstates $|n_1\rangle$ and $|n_2\rangle$ of the number operators $n_1 = a_1^\dagger a_1$ and $n_2 = a_2^\dagger a_2$ in the usual way : $a_1 |n_1\rangle = \sqrt{n_1}\,|n_1 - 1\rangle$, $a_1^\dagger |n_1\rangle = \sqrt{n_1+1}\,|n_1+1\rangle$, $n_1 |n_1\rangle = n_1 |n_1\rangle$ and similarly for $a_2$. In terms of $a_1$ and $a_2$, $H_0$ becomes

$$H_0 = \hbar\omega_l \left(a_1^\dagger a_1 + a_2^\dagger a_2 + 1\right) + \frac{\hbar\omega_c}{2}\left(a_1^\dagger a_1 - a_2^\dagger a_2\right) + \frac{\alpha_0}{\lambda^2}\frac{\tilde{g}}{2}\sigma_z, \tag{59}$$

which directly leads to its eigenvalues

$$E_{n_1,n_2,\sigma} = \hbar\omega_l\,(n_1 + n_2 + 1) + \frac{\hbar\omega_c}{2}\,(n_1 - n_2) + \frac{\alpha_0}{\lambda^2}\frac{\tilde{g}}{2}\sigma \tag{60}$$

and corresponding eigenstates $|n_1, n_2, \sigma\rangle$ with $n_{1,2} = \{0, 1, 2, \dots\}$ and $\sigma = \pm 1$.

The set of eigenstates of $H_0$ defines an orthonormal basis on which we can project $H'$. The spin-orbit term $H'$ depends on products and powers of the $K_\pm$ operators (eq. (2) in main text). The matrix expression for $H'$ in the $\{|n_1, n_2, \sigma\rangle\}$ basis can be found from the expression of $K_\pm$ in terms of $a_1$ and $a_2$ :

$$K_- = -i\kappa_+ a_1 + i\kappa_- a_2^\dagger, \tag{61}$$

$$K_\parallel^2 = \frac{1}{2}\{K_-, K_+\}, \tag{62}$$

where $\kappa_\pm = 1/r \pm r/(2\lambda^2)$. We cannot however perform the projection on every basis states $|n_1, n_2, \sigma\rangle$ because $H_{\text{eff}}$ diverges from the exact dispersion $H_\parallel$ at some point. Thus, the projection is done only on the finite subset $n_1 + n_2 \leq 4$. The size of this truncated basis subset is chosen large enough to include the orbitals from the $n_1 + n_2 = 1$

and $n_1+n_2=3$ groups that have a significant contribution in $|\mathbb{0}\rangle$ and $|\mathbb{1}\rangle$ [5, 6], but small enough that the expectation value

$$\sqrt{\left\langle K_{\|}^2\right\rangle}=\sqrt{(n_1+1/2)\kappa_+^2+(n_2+1/2)\kappa_-^2} \tag{63}$$

is smaller than the point in $k$-space where $H_{\rm eff}(\mathbf{K}_{\|})$ diverges from $H_{\|}$ too significantly.

The qubit levels $|\mathbb{0}\rangle$ and $|\mathbb{1}\rangle$ can be expanded in terms of the Fock-Darwin orbitals $|n_1,n_2,\sigma\rangle$ using perturbation theory :

$$|\mathbb{0}\rangle=|0,0,-\rangle-\frac{\kappa_-\beta'}{E_{0,0,-}-E_{0,1,+}}|0,1,+\rangle-\frac{\sqrt{6}\kappa_+^3\beta_2}{E_{0,0,-}-E_{3,0,+}}|3,0,+\rangle+\frac{\sqrt{2}\kappa_-^2\kappa_+\beta_3}{E_{0,0,-}-E_{1,2,+}}|1,2,+\rangle \tag{64}$$

$$|\mathbb{1}\rangle=|0,0,+\rangle+\frac{\kappa_+\beta'}{E_{0,0,+}-E_{1,0,-}}|1,0,-\rangle+\frac{\sqrt{6}\kappa_-^3\beta_2}{E_{0,0,+}-E_{0,3,-}}|0,3,-\rangle-\frac{\sqrt{2}\kappa_+^2\kappa_-\beta_3}{E_{0,0,+}-E_{2,1,-}}|2,1,-\rangle, \tag{65}$$

where $\beta'=\beta_1+(\kappa_+^2+\kappa_-^2)\beta_3$. These expressions are valid only far away from any crossing between Fock-Darwin states that would make a denominator vanish.

For reference, the full Hamiltonian $H_{\rm QD}$ in terms of $a_{1,2}$ (neglecting $K^4$ anisotropy and non-parabolicity terms) is given by

$$\begin{aligned}H_{\rm QD} &=\hbar\omega_l\left(a_1^\dagger a_1+a_2^\dagger a_2+1\right)+\frac{\hbar\omega_c}{2}\left(a_1^\dagger a_1-a_2^\dagger a_2\right)+\frac{\alpha_0}{\lambda^2}\frac{\tilde g}{2}\sigma_z+\frac{\alpha_0^2}{\lambda^4}\tilde g'\\ &+\frac{\alpha_0^2}{\lambda^2}\gamma_\lambda\left[\kappa_+^2\left(a_1^\dagger a_1+\frac12\right)+\kappa_-^2\left(a_2^\dagger a_2+\frac12\right)-\kappa_+\kappa_-\left(a_1a_2+a_1^\dagger a_2^\dagger\right)\right]\sigma_z\\ &+\beta_1\left[\left(\kappa_+a_1-\kappa_-a_2^\dagger\right)\sigma_++h.c.\right]-\beta_2\left[\left(\kappa_+^3a_1^{\dagger3}-3\kappa_+^2\kappa_-a_1^{\dagger2}a_2+3\kappa_+\kappa_-^2a_1^\dagger a_2^2-\kappa_-^3a_2^3\right)\sigma_++h.c.\right]\\ &+\beta_3\left\{\left[\kappa_+^3a_1a_1^\dagger a_1-\kappa_+^2\kappa_-\left(a_1^2a_2+(2a_1^\dagger a_1+1)a_2^\dagger\right)+\kappa_+\kappa_-^2\left(a_1(2a_2^\dagger a_2+1)+a_1^\dagger a_2^{\dagger2}\right)-\kappa_-^3a_2^\dagger a_2a_2^\dagger\right]\sigma_++h.c.\right\}\end{aligned} \tag{66}$$

## LIGHT HOLE-PHONON INTERACTION

We estimate the relaxation time $T_1$ of the qubit by evaluating the rate of the single phonon-mediated qubit transitions :

$$\Gamma_i=\frac{2\pi\mathcal{V}}{\hbar}\sum_\alpha\int\frac{d^3q}{(2\pi)^3}\left|\langle f|W_\alpha|i\rangle\right|^2\delta(\hbar\omega-\hbar\omega_{\alpha\mathbf{q}}). \tag{67}$$

For absorption, $|i\rangle=|\mathbb{0}\rangle|{\rm TP}\rangle$ and $|f\rangle=b_{\alpha\mathbf{q}}|\mathbb{1}\rangle|{\rm TP}\rangle/\sqrt{N_{\alpha\mathbf{q}}}$ while for emission, $|i\rangle=|\mathbb{1}\rangle|{\rm TP}\rangle$ and $|f\rangle=b_{\alpha,-\mathbf{q}}^\dagger|\mathbb{0}\rangle|{\rm TP}\rangle/\sqrt{N_{\alpha,-\mathbf{q}}+1}$. Here, $|{\rm TP}\rangle$ is the thermal phonon bath with $b_{\alpha\mathbf{q}}^\dagger b_{\alpha\mathbf{q}}|{\rm TP}\rangle=N_{\alpha\mathbf{q}}|{\rm TP}\rangle$, where $N_{\alpha\mathbf{q}}=1/\left(e^{\hbar\omega_{\alpha\mathbf{q}}/k_{\rm B}T}-1\right)$ is the phonon occupation number. The delta function can be eliminated for each polarization by setting $q=q_\alpha=\omega/v_\alpha$, which gives

$$\Gamma_i=\frac{\mathcal{V}}{(2\pi)^2}\left(\frac{\omega}{\hbar}\right)^2\sum_\alpha\frac{1}{v_\alpha^3}\int\sin\theta d\theta d\phi\left|\langle f|W_\alpha|i\rangle\right|^2, \tag{68}$$

where $v_{\rm LA}=\sqrt{c_{11}/\rho}$ and $v_{\rm TA}=\sqrt{c_{44}/\rho}$. The $W_\alpha$ operator derives from the hole-phonon Hamiltonian which is given by (16) but with the strain tensor given by [7, 8]

$$\varepsilon_{\alpha\mathbf{q}} = iq\sqrt{\frac{A_\alpha}{q}} e^{i\mathbf{q}\cdot\mathbf{r}} \left(b_{\alpha\mathbf{q}} + b^\dagger_{\alpha,-\mathbf{q}}\right) \epsilon_{\alpha\mathbf{q}}, \tag{69}$$

with $A_\alpha = \hbar/(2\rho\mathcal{V}v_\alpha)$ and

$$\epsilon_{\alpha\mathbf{q}} = \frac{1}{2}\begin{bmatrix} 2\hat{c}_x\hat{q}_x & \hat{c}_x\hat{q}_y + \hat{c}_y\hat{q}_x & \hat{c}_x\hat{q}_z + \hat{c}_z\hat{q}_x \\ \hat{c}_y\hat{q}_x + \hat{c}_x\hat{q}_y & 2\hat{c}_y\hat{q}_y & \hat{c}_y\hat{q}_z + \hat{c}_z\hat{q}_y \\ \hat{c}_z\hat{q}_x + \hat{c}_x\hat{q}_z & \hat{c}_z\hat{q}_y + \hat{c}_y\hat{q}_z & 2\hat{c}_z\hat{q}_z \end{bmatrix} \tag{70}$$

with $\hat{\mathbf{c}}_{\alpha\mathbf{q}}$ the unit polarization vector and $\hat{\mathbf{q}} = \mathbf{q}/q$. We write the hole-phonon Hamiltonian along with $H_\parallel$ onto the $\{\eta+, \eta-, \mathrm{H}+, \mathrm{H}-\}$ subband edge basis before we perform a 2nd order Schrieffer-Wolff transformation to find an effective Hamiltonian for the LH-phonon interaction in the qubit subspace. We keep only terms that are linear in $b_{\alpha\mathbf{q}}$. This gives

$$W_\alpha = i\sqrt{q}\left(b_{\alpha\mathbf{q}} + b^\dagger_{\alpha,-\mathbf{q}}\right)\left(W_{11}\sigma_+\sigma_- + W_{22}\sigma_-\sigma_+ + W_{12}\sigma_+ + W_{21}\sigma_-\right). \tag{71}$$

The expressions for $W_{ij}$ are quite lengthy, so here we give as an example the result of the product $\langle \mathbb{1} \,|\, W_{11}\sigma_+\sigma_- \,|\, \mathbb{0}\rangle$ :

$$\langle \mathbb{1} \,|\, W_{11}\sigma_+\sigma_- \,|\, \mathbb{0}\rangle = c^{\mathbb{1}*}_{0,0} w^\alpha_{\eta+\eta+}\left(c^{\mathbb{0}}_{0,1}e_{02} + c^{\mathbb{0}}_{1,2}e_{05} + c^{\mathbb{0}}_{3,0}e_{03}\right) + i\kappa_-\left(\frac{\mathbf{w}^\alpha_{\eta+\eta-}\mathbf{R}}{\mathbf{\Delta}_{\eta\eta}} + \frac{\mathbf{P}\mathbf{w}^\alpha_{\mathrm{H}+\eta+}}{\mathbf{\Delta}_{\eta\mathrm{H}}}\right) c^{\mathbb{1}*}_{0,0}c^{\mathbb{0}}_{0,1}, \tag{72}$$

The relevant $\mathbf{w}^\alpha_{AB}$ matrix elements are :

$$w^{\mathrm{LA}}_{\eta+\eta+} = w^{\mathrm{LA}}_{\eta-\eta-} = {}_c\langle j \,|\, a'_c \,|\, j'\rangle_c + \frac{2}{3}\,{}_-\big\langle j \,\big|\, a'_v - b'(1-3\cos^2\theta) \,\big|\, j'\big\rangle_- + \frac{1}{6}\,{}_+\big\langle j \,\big|\, 2a'_v + b'(1-3\cos^2\theta) \,\big|\, j'\big\rangle_+ \tag{73}$$

$$w^{\mathrm{LA}}_{\eta+\eta-} = \frac{\sin 2\theta e^{-i\phi}}{2\sqrt{3}}\left({}_-\langle j \,|\, d' \,|\, j'\rangle_+ - {}_+\langle j \,|\, d' \,|\, j'\rangle_-\right) \tag{74}$$

$$w^{\mathrm{LA}}_{\mathrm{H}+\eta+} = -\frac{\sin 2\theta e^{-i\phi}}{2}\,{}_h\langle l \,|\, d' \,|\, j\rangle_- \tag{75}$$

$$w^{\mathrm{TA1}}_{\eta+\eta+} = w^{\mathrm{TA1}}_{\eta-\eta-} = \sin 2\theta\left(\frac{1}{4}\,{}_+\langle j \,|\, b' \,|\, j'\rangle_+ - {}_-\langle j \,|\, b' \,|\, j'\rangle_-\right) \tag{76}$$

$$w^{\mathrm{TA1}}_{\eta+\eta-} = \frac{\cos 2\theta e^{-i\phi}}{2\sqrt{3}}\left({}_-\langle j \,|\, d' \,|\, j'\rangle_+ - {}_+\langle j \,|\, d' \,|\, j'\rangle_-\right) \tag{77}$$

$$w^{\mathrm{TA1}}_{\mathrm{H}+\eta+} = -\frac{\cos 2\theta e^{-i\phi}}{2}\,{}_h\langle l \,|\, d' \,|\, j\rangle_- \tag{78}$$

$$w^{\mathrm{TA2}}_{\eta+\eta+} = w^{\mathrm{TA2}}_{\eta-\eta-} = 0 \tag{79}$$

$$w^{\mathrm{TA2}}_{\eta+\eta-} = -i\frac{\cos 2\theta e^{-i\phi}}{2\sqrt{3}}\left({}_-\langle j \,|\, d' \,|\, j'\rangle_+ - {}_+\langle j \,|\, d' \,|\, j'\rangle_-\right) \tag{80}$$

$$w^{\mathrm{TA2}}_{\mathrm{H}+\eta+} = \frac{i\cos 2\theta e^{-i\phi}}{2}\,{}_h\langle l \,|\, d' \,|\, j\rangle_-\,, \tag{81}$$

where $a'_c = a_c\sqrt{A_\alpha}e^{iqz\cos\theta}$ and similarly for $a'_v$, $b'$ and $d'$. We make the assumption $e^{iqz\cos\theta} \approx 1$ in the 2nd order terms $\mathbf{w}^\alpha_{\eta+\eta-}\mathbf{R}/\mathbf{\Delta}_{\eta\eta}$ and alike.

The braket products involving $e^{i\mathbf{q}_\parallel\cdot\mathbf{r}_\parallel}$, where $\mathbf{r}_\parallel = x\mathbf{e}_x + y\mathbf{e}_y$, are calculated analytically from the expressions of $|n_1, n_2\rangle$ in position space :

$$\phi_{0,0}(x,y) = \frac{1}{\sqrt{\pi}r} e^{-\left(x^2+y^2\right)/\left(2r^2\right)} \tag{82}$$

$$\phi_{1,0}(x,y) = \phi^*_{0,1}(x,y) = \frac{x+iy}{r}\phi_{0,0}(x,y) \tag{83}$$

$$\phi_{3,0}(x,y) = \phi^*_{0,3}(x,y) = \frac{(x+iy)^3}{\sqrt{6}r^3}\phi_{0,0}(x,y) \tag{84}$$

$$\phi_{2,1}(x,y) = \phi^*_{1,2}(x,y) = \frac{x+iy}{\sqrt{2}r}\left(\frac{x^2+y^2}{r^2} - 2\right)\phi_{0,0}(x,y). \tag{85}$$

If we define $|0\rangle \equiv |0,0\rangle$, $|1\rangle \equiv |1,0\rangle$, $|2\rangle \equiv |0,1\rangle$, $|3\rangle \equiv |3,0\rangle$, $|4\rangle \equiv |2,1\rangle$, $|5\rangle \equiv |1,2\rangle$ and $|6\rangle \equiv |0,3\rangle$ with $e_{ab} \equiv \left\langle a \middle| e^{i\mathbf{q}_\parallel \cdot \mathbf{r}_\parallel} \middle| b \right\rangle$ we have :

$$e_{01} = \frac{it}{2}e^{i\phi}e_{00} \qquad e_{02} = e^*_{01}(-q) \qquad e_{03} = -\frac{it^3}{8\sqrt{6}}e^{3i\phi}e_{00}$$

$$e_{04} = -\frac{it^3}{8\sqrt{2}}e^{i\phi}e_{00} \qquad e_{05} = e^*_{04}(-q) \qquad e_{06} = e^*_{03}(-q)$$

$$e_{12} = -\frac{t^2}{4}e^{-2i\phi}e_{00} \qquad e_{13} = -\frac{3t^2}{4\sqrt{6}}\left(1-\frac{t^2}{12}\right)e^{2i\phi}e_{00} \qquad e_{15} = -\frac{t^2}{4\sqrt{2}}\left(1-\frac{t^2}{4}\right)e^{-2i\phi}e_{00}$$

$$e_{24} = e^*_{15} \qquad e_{26} = e^*_{13} \qquad e_{34} = -\frac{\sqrt{3}t^2}{4}\left[1-\frac{t^2}{4}\left(1-\frac{t^2}{24}\right)\right]e^{-2i\phi}e_{00}$$

$$e_{36} = -\frac{t^2}{384}e^{-6i\phi}e_{00} \qquad e_{45} = -\frac{t^2}{2}\left(1-\frac{t^2}{8}\right)^2 e^{-2i\phi}e_{00} \qquad e_{56} = e_{34},$$

where $t = qr\sin\theta$ and $e_{00} = e^{-t^2/4}$.

## MATERIAL PARAMETRIZATION

The material parameters of $Ge_{1-x}Sn_x$ are obtained from a linear interpolation between those of pure Ge and pure Sn. A bowing parameter is also incorporated if necessary :

$$A(x) = (1-x)A^{\mathrm{Ge}} + xA^{\mathrm{Sn}} - x(1-x)b^A. \tag{86}$$

Table I lists the parameters that were used in the calculations. The Luttinger parameters $\gamma_{1,2,3}$ are an exception to the interpolation scheme, as they are evaluated by interpolating their values from pure Ge and from GeSn at $x = 20\%$ Sn :

$$\gamma(x) = \left(1-\frac{x}{0.2}\right)\gamma^{\mathrm{Ge}} + \frac{x}{0.2}\gamma^{\mathrm{GeSn}} - \frac{x}{0.2}\left(1-\frac{x}{0.2}\right)b^\gamma. \tag{87}$$

TABLE I. Input parameters with bowings for the 8-band $k \cdot p$ model.

| Parameter | Germanium | Tin | Bowing |
|---|---|---|---|
| Lattice constant | | | |
| $a_0$ (Å, 0 K) | 5.652357[a] | 6.480117[b] | −0.083[c] |
| Energy gaps | | | |
| $E_g$ (eV, 0 K) | 0.8981[d] | −0.39[e] | 2.46[e] |
| $\Delta$ (eV) | 0.289[c] | 0.600[c] | −0.100[c] |
| $E_{v,\mathrm{avg}}$ (eV) | 0 | 0.69[g] | |
| Elastic constants and density | | | |
| $c_{11}$ (GPa) | 128.53[d] | 69.00[g] | |
| $c_{12}$ (GPa) | 48.28[d] | 29.30[g] | |
| $c_{44}$ (GPa) | 66.80[d] | 36.20[g] | |
| $\rho$ (g/cm$^3$) | 5.323[b] | 7.285[b] | |
| Deformation potentials[†] | | | |
| $a_{c\Gamma}$ (eV) | −10.41[d] | −6.00[g] | |
| $a_v$ (eV) | 1.24[d] | 1.58[g] | |
| $b$ (eV) | −2.86[d] | −2.7[g] | |
| $d$ (eV) | −5.28[d] | −4.1[b] | |
| Effective mass and spin parameters | | | |
| $m_c$ ($m_0$) | 0.0383[d] | −0.058[f] | |
| $\gamma_1^{\mathrm{L}}$ | 13.37[d] | 29.21[h*] | 20.34[h] |
| $\gamma_2^{\mathrm{L}}$ | 4.23[d] | 12.24[h*] | 9.66[h] |
| $\gamma_3^{\mathrm{L}}$ | 5.68[d] | 13.74[h*] | 9.82[h] |
| $\kappa^{\mathrm{L}}$ | 3.41[f] | −11.84[f] | |
| $g_c$ | −2.86[f] | 84.4[f] | |
| $E_p$ (eV) | 26.3[d] | 24.0[g] | |

[†] The convention $a = a_c - a_v$ is used.
[*] Values for $Ge_{0.8}Sn_{0.2}$.
[a] Reference 9
[b] Reference 10
[c] Reference 11
[d] Reference 12
[e] Reference 13
[f] Reference 14
[g] Reference 15
[h] Reference 16

* oussama.moutanabbir@polymtl.ca

[1] T. Eißfeller, *Theory of the electronic structure of quantum dots in external fields*, Ph.D. thesis, Technische Universitaet Muenchen (Germany) (2012).
[2] B. A. Foreman, Elimination of spurious solutions from eight-band $\mathbf{k} \cdot \mathbf{p}$ theory, Phys. Rev. B **56**, R12748 (1997).
[3] R. Winkler, *Spin-orbit coupling effects in two-dimensional electron and hole systems*, Springer tracts in modern physics (Springer, Berlin, 2003).
[4] C. G. Van de Walle, Band lineups and deformation potentials in the model-solid theory, Phys. Rev. B **39**, 1871 (1989).
[5] D. V. Bulaev and D. Loss, Spin Relaxation and Decoherence of Holes in Quantum Dots, Phys. Rev. Lett. **95**, 076805 (2005).
[6] L. A. Terrazos, E. Marcellina, Z. Wang, S. N. Coppersmith, M. Friesen, A. R. Hamilton, X. Hu, B. Koiller, A. L. Saraiva, D. Culcer, and R. B. Capaz, Theory of hole-spin qubits in strained germanium quantum dots, Phys. Rev. B **103**, 125201 (2021).
[7] J. Li, B. Venitucci, and Y.-M. Niquet, Hole-phonon interactions in quantum dots: Effects of phonon confinement and encapsulation materials on spin-orbit qubits, Phys. Rev. B **102**, 075415 (2020).
[8] L. M. Woods, T. L. Reinecke, and R. Kotlyar, Hole spin relaxation in quantum dots, Phys. Rev. B **69**, 125330 (2004).
[9] R. R. Reeber and K. Wang, Thermal expansion and lattice parameters of group IV semiconductors, Materials Chemistry and Physics **46**, 259 (1996).
[10] O. Madelung, ed., *Semiconductors, Group IV Elements and III-V Compounds* (Springer-Verlag Berlin Heidelberg, 1991).
[11] M. P. Polak, P. Scharoch, and R. Kudrawiec, The electronic band structure of Ge1-xSnxin the full composition range: indirect, direct, and inverted gaps regimes, band offsets, and the Burstein–Moss effect, Journal of Physics D: Applied Physics **50**, 195103 (2017).
[12] D. J. Paul, 8-band $\mathbf{k}\cdot\mathbf{p}$ modelling of mid-infrared intersubband absorption in Ge quantum wells, Journal of Applied Physics **120**, 043103 (2016), https://doi.org/10.1063/1.4959259.
[13] M. Bertrand, Q.-M. Thai, J. Chrétien, N. Pauc, J. Aubin, L. Milord, A. Gassenq, J.-M. Hartmann, A. Chelnokov, V. Calvo, and V. Reboud, Experimental Calibration of Sn-Related Varshni Parameters for High Sn Content GeSn Layers, Annalen der Physik **531**, 1800396 (2019), https://onlinelibrary.wiley.com/doi/pdf/10.1002/andp.201800396.
[14] P. Lawaetz, Valence-Band Parameters in Cubic Semiconductors, Phys. Rev. B **4**, 3460 (1971).
[15] G. Chang, S. Chang, and S. L. Chuang, Strain-Balanced $Ge_zSn_{1-z}$–$Si_xGe_ySn_{1-x-y}$ Multiple-Quantum-Well Lasers, IEEE Journal of Quantum Electronics **46**, 1813 (2010).
[16] K. Lu Low, Y. Yang, G. Han, W. Fan, and Y.-C. Yeo, Electronic band structure and effective mass parameters of Ge1-xSnx alloys, Journal of Applied Physics **112**, 103715 (2012), https://doi.org/10.1063/1.4767381.
